# Supplementary material for: Semantic Scene Completion via Integrating Instances and Scene in-the-Loop
Source: arXiv:2104.03640 source file (2021-06-06)
Supplement: Supplementary file 1 [file supp-vis.tex]

\begin{table}[ht]
\begin{center}
\resizebox{0.48\textwidth}{!}{
\begin{tabular}{|l| c|c c|c c|} 
\hline
\textbf{Methods}& \textbf{Dataset}& \multicolumn{2}{c|}{\textbf{Visible}} & \multicolumn{2}{c|}{\textbf{Invisible}} \\ \hline
  & &SC & SSC & SC & SSC \\ 
\hline
Baseline &NYU& 98.1 & 47.3 & 64.5 & 38.7 \\ \hline
+\textit{S-I-S Once} &NYU& 97.6 & 53.6 & 70.9 & 45.3 \\ \hline
+\textit{Iter S-I-S} &NYU& \textbf{98.1} & \textbf{55.5} & \textbf{72.3} & \textbf{46.8} \\ \hline
\hline
Baseline &NYUCAD& 99.6 & 62.2 & 80.7 & 49.1 \\ \hline
+\textit{S-I-S Once} &NYUCAD& 99.6 & 68.2 & 84.1 & 54.9 \\ \hline
+\textit{Iter S-I-S} &NYUCAD& \textbf{99.6} & \textbf{69.5} & \textbf{84.7} & \textbf{56.3} \\ \hline
\hline
Baseline &SUNCG-RGBD& 93.5 & 85.6 & 86.2 & 59.0 \\ \hline
+\textit{S-I-S Once} &SUNCG-RGBD& 95.9 & 88.1 & 88.9 & 64.4 \\ \hline
+\textit{Iter S-I-S} &SUNCG-RGBD& \textbf{96.3} & \textbf{88.4} & \textbf{88.9} & \textbf{65.0} \\ \hline
\end{tabular}
}
% \vspace{-0.6cm}
\end{center}
\vspace{-0.2cm}
%\caption{\textbf{Results on NYU dataset}. Bold numbers represent the best scores. \textit{Resolution(a, b)} means the input and output resolution is $(a \times 0.6a \times a)$ and the output resolution is $(b \times 0.6b \times b)$.}
\caption{\textbf{Visible and Invisible Region Results of the three datastes}. Bold numbers represent the best scores.}
\label{tab:supp-vis}
%\vspace{-0.3cm}
\end{table}
